# Supplementary material for: One-Shot Learning of Multi-Step Tasks from Observation via Activity Localization in Auxiliary Video
Source: arXiv:1806.11244 source file (2019-04-26)
Supplement: Supplementary file 2 [file appendix.tex]

\WJ{TODO: Breakfast / NIV Examples}

\begin{figure*}
    \centering
    \includegraphics[width=\textwidth]{assets/sample_reacher.png}
    \includegraphics[width=\textwidth]{assets/sample_reacher_meta.png}
    \caption{
        Demonstration videos for reacher task. Sample video from training set \textbf{(top)} and meta-test \textbf{(bottom)}.
        Each of the video contains a video reaching to two multiple targets; (\textcolor{orange}{orange}, \textcolor{green}{green}) for training set, and (\textcolor{SpringGreen}{light green}, \textcolor{Fuchsia}{purple}) for meta-test set. Rest two colors are distractors.
    }
    \label{fig:task_example}
\end{figure*}

\WJ{TODO: Network Architecture}

\begin{figure*}[!htbp]
    \centering
    \includegraphics[width=\textwidth]{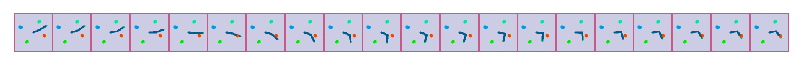}\\
    \includegraphics[width=\textwidth]{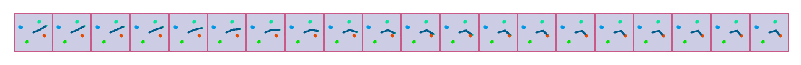}\\
    \includegraphics[width=\textwidth]{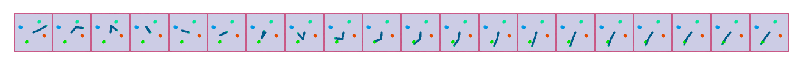}\\
    \includegraphics[width=\textwidth]{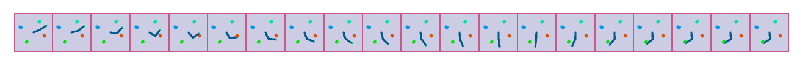}
    \caption{
        The successful roll-outs of 4 different policies. Each strip represents an execution of policies for action orange and green in an identical setting. The two strips on the top is the result for reaching to orange with MAML-aligned video segments and perfectly aligned video segments. The two strips on the bottom is the result for reaching to green. While all 4 executions succeed, but it is noticeable that the policy trained with the reward function trained with perfectly aligned videos generate more stable policies.
    }
    \label{fig:RL_Results}
\end{figure*}

\subsection{Breakfast Validation Set - Qualitative Results}

A target task and a legend for each color is shown on top.
Each color strip represents ground truth, predicted alignmented, and correctness from the top to bottom.
The pair of a demonstration video and a target sample video is choosen randomly.
From the left to the right, each column represents the result of meta learning method, triplet method, and classifier baseline.

\begin{figure}[!htbp]
  \centering
  \includegraphics[width=0.85\linewidth,keepaspectratio]{./assets/bf_qual/output_2_0.png}\\
  \includegraphics[width=0.85\linewidth,keepaspectratio]{./assets/bf_qual/output_2_1.png}\\
  \includegraphics[width=0.85\linewidth,keepaspectratio]{./assets/bf_qual/output_2_2.png}\\
  \includegraphics[width=0.85\linewidth,keepaspectratio]{./assets/bf_qual/output_2_3.png}\\
  \includegraphics[width=0.85\linewidth,keepaspectratio]{./assets/bf_qual/output_2_4.png}\\
  %\label{}
\end{figure}
\begin{figure}[!htbp]
  \centering
  \includegraphics[width=0.85\linewidth,keepaspectratio]{./assets/bf_qual/output_2_5.png}\\
  \includegraphics[width=0.85\linewidth,keepaspectratio]{./assets/bf_qual/output_2_6.png}\\
  \includegraphics[width=0.85\linewidth,keepaspectratio]{./assets/bf_qual/output_2_7.png}\\
  \includegraphics[width=0.85\linewidth,keepaspectratio]{./assets/bf_qual/output_2_8.png}\\
  \includegraphics[width=0.85\linewidth,keepaspectratio]{./assets/bf_qual/output_2_9.png}\\
  %\label{}
\end{figure}
\begin{figure}[!htbp]
  \centering
  \includegraphics[width=0.9\linewidth,keepaspectratio]{./assets/bf_qual/output_2_10.png}\\
  \includegraphics[width=0.9\linewidth,keepaspectratio]{./assets/bf_qual/output_2_11.png}\\
  \includegraphics[width=0.9\linewidth,keepaspectratio]{./assets/bf_qual/output_2_12.png}\\
  \includegraphics[width=0.9\linewidth,keepaspectratio]{./assets/bf_qual/output_2_13.png}\\
  \includegraphics[width=0.9\linewidth,keepaspectratio]{./assets/bf_qual/output_2_14.png}\\
  %\label{}
\end{figure}
\begin{figure}[!htbp]
  \centering
  \includegraphics[width=0.9\linewidth,keepaspectratio]{./assets/bf_qual/output_2_15.png}\\
  \includegraphics[width=0.9\linewidth,keepaspectratio]{./assets/bf_qual/output_2_16.png}\\
  \includegraphics[width=0.9\linewidth,keepaspectratio]{./assets/bf_qual/output_2_17.png}\\
  \includegraphics[width=0.9\linewidth,keepaspectratio]{./assets/bf_qual/output_2_18.png}\\
  \includegraphics[width=0.9\linewidth,keepaspectratio]{./assets/bf_qual/output_2_19.png}\\
  %\label{}
\end{figure}
\begin{figure}[!htbp]
  \centering
  \includegraphics[width=0.9\linewidth,keepaspectratio]{./assets/bf_qual/output_2_20.png}\\
  \includegraphics[width=0.9\linewidth,keepaspectratio]{./assets/bf_qual/output_2_21.png}\\
  \includegraphics[width=0.9\linewidth,keepaspectratio]{./assets/bf_qual/output_2_22.png}\\
  \includegraphics[width=0.9\linewidth,keepaspectratio]{./assets/bf_qual/output_2_23.png}\\
  \includegraphics[width=0.9\linewidth,keepaspectratio]{./assets/bf_qual/output_2_24.png}\\
  %\label{}
\end{figure}
\begin{figure}[!htbp]
  \centering
  \includegraphics[width=0.9\linewidth,keepaspectratio]{./assets/bf_qual/output_2_25.png}\\
  \includegraphics[width=0.9\linewidth,keepaspectratio]{./assets/bf_qual/output_2_26.png}\\
  \includegraphics[width=0.9\linewidth,keepaspectratio]{./assets/bf_qual/output_2_27.png}\\
  \includegraphics[width=0.9\linewidth,keepaspectratio]{./assets/bf_qual/output_2_28.png}\\
  \includegraphics[width=0.9\linewidth,keepaspectratio]{./assets/bf_qual/output_2_29.png}\\
  %\label{}
\end{figure}
\begin{figure}[!htbp]
  \centering
  \includegraphics[width=0.9\linewidth,keepaspectratio]{./assets/bf_qual/output_2_30.png}\\
  \includegraphics[width=0.9\linewidth,keepaspectratio]{./assets/bf_qual/output_2_31.png}\\
  \includegraphics[width=0.9\linewidth,keepaspectratio]{./assets/bf_qual/output_2_32.png}\\
  \includegraphics[width=0.9\linewidth,keepaspectratio]{./assets/bf_qual/output_2_33.png}\\
  \includegraphics[width=0.9\linewidth,keepaspectratio]{./assets/bf_qual/output_2_34.png}\\
  %\label{}
\end{figure}

\clearpage

\subsection{Breakfast Meta-Test Set - Qualitative Results}

\begin{figure}[!htbp]
  \centering
  \includegraphics[width=0.9\linewidth,keepaspectratio]{./assets/bf_qual/output_1_0.png}\\
  \includegraphics[width=0.9\linewidth,keepaspectratio]{./assets/bf_qual/output_1_1.png}\\
  \includegraphics[width=0.9\linewidth,keepaspectratio]{./assets/bf_qual/output_1_2.png}\\
  \includegraphics[width=0.9\linewidth,keepaspectratio]{./assets/bf_qual/output_1_3.png}\\
  \includegraphics[width=0.9\linewidth,keepaspectratio]{./assets/bf_qual/output_1_4.png}\\
  \includegraphics[width=0.9\linewidth,keepaspectratio]{./assets/bf_qual/output_1_5.png}\\
  \includegraphics[width=0.9\linewidth,keepaspectratio]{./assets/bf_qual/output_1_6.png}\\
  \includegraphics[width=0.9\linewidth,keepaspectratio]{./assets/bf_qual/output_1_7.png}\\
  \includegraphics[width=0.9\linewidth,keepaspectratio]{./assets/bf_qual/output_1_8.png}\\
  \includegraphics[width=0.9\linewidth,keepaspectratio]{./assets/bf_qual/output_1_9.png}\\
  %\label{}
\end{figure}

\begin{figure}[!htbp]
  \centering
  \includegraphics[width=0.9\linewidth,keepaspectratio]{./assets/bf_qual/output_1_11.png}\\
  \includegraphics[width=0.9\linewidth,keepaspectratio]{./assets/bf_qual/output_1_12.png}\\
  \includegraphics[width=0.9\linewidth,keepaspectratio]{./assets/bf_qual/output_1_13.png}\\
  \includegraphics[width=0.9\linewidth,keepaspectratio]{./assets/bf_qual/output_1_14.png}\\
  \includegraphics[width=0.9\linewidth,keepaspectratio]{./assets/bf_qual/output_1_15.png}\\
  \includegraphics[width=0.9\linewidth,keepaspectratio]{./assets/bf_qual/output_1_16.png}\\
  \includegraphics[width=0.9\linewidth,keepaspectratio]{./assets/bf_qual/output_1_17.png}\\
  \includegraphics[width=0.9\linewidth,keepaspectratio]{./assets/bf_qual/output_1_18.png}\\
  \includegraphics[width=0.9\linewidth,keepaspectratio]{./assets/bf_qual/output_1_20.png}\\
  \includegraphics[width=0.9\linewidth,keepaspectratio]{./assets/bf_qual/output_1_21.png}\\
  %\label{}
\end{figure}

\begin{figure}[!htbp]
  \centering
  \includegraphics[width=0.9\linewidth,keepaspectratio]{./assets/bf_qual/output_1_22.png}\\
  \includegraphics[width=0.9\linewidth,keepaspectratio]{./assets/bf_qual/output_1_23.png}\\
  \includegraphics[width=0.9\linewidth,keepaspectratio]{./assets/bf_qual/output_1_24.png}\\
  \includegraphics[width=0.9\linewidth,keepaspectratio]{./assets/bf_qual/output_1_26.png}\\
  \includegraphics[width=0.9\linewidth,keepaspectratio]{./assets/bf_qual/output_1_27.png}\\
  \includegraphics[width=0.9\linewidth,keepaspectratio]{./assets/bf_qual/output_1_28.png}\\
  \includegraphics[width=0.9\linewidth,keepaspectratio]{./assets/bf_qual/output_1_29.png}\\
  \includegraphics[width=0.9\linewidth,keepaspectratio]{./assets/bf_qual/output_1_30.png}\\
  \includegraphics[width=0.9\linewidth,keepaspectratio]{./assets/bf_qual/output_1_31.png}\\
  \includegraphics[width=0.9\linewidth,keepaspectratio]{./assets/bf_qual/output_1_32.png}\\
  %\label{}
\end{figure}

\clearpage

\subsection{Breakfast Validation Set - Triplet Network Deatiled Alignment Analysis}

To take a deep look at how alignments is made by triplet network method,
distances between every pair of video segments is plotted below.
The white area represents low distance (more similar) and vice versa.
The picked segment in demonstration video for alignments (a segment having the lowest distance) for every sample video segment
is visualized in a red dot.

\begin{figure}[!htbp]
  \centering
  \includegraphics[width=0.9\linewidth,keepaspectratio]{./assets/bf_qual/output_3_0.png}\\
  \includegraphics[width=0.45\linewidth,keepaspectratio]{./assets/bf_qual/output_3_1.png}
  \includegraphics[width=0.45\linewidth,keepaspectratio]{./assets/bf_qual/output_3_2.png}
  \includegraphics[width=0.45\linewidth,keepaspectratio]{./assets/bf_qual/output_3_3.png}
  \includegraphics[width=0.45\linewidth,keepaspectratio]{./assets/bf_qual/output_3_4.png}
  \includegraphics[width=0.45\linewidth,keepaspectratio]{./assets/bf_qual/output_3_5.png}
  \includegraphics[width=0.45\linewidth,keepaspectratio]{./assets/bf_qual/output_3_6.png}
  %\label{}
\end{figure}

\begin{figure}[!htbp]
  \centering
  \includegraphics[width=0.9\linewidth,keepaspectratio]{./assets/bf_qual/output_3_7.png}\\
  \includegraphics[width=0.45\linewidth,keepaspectratio]{./assets/bf_qual/output_3_8.png}
  \includegraphics[width=0.45\linewidth,keepaspectratio]{./assets/bf_qual/output_3_9.png}
  \includegraphics[width=0.45\linewidth,keepaspectratio]{./assets/bf_qual/output_3_10.png}
  \includegraphics[width=0.45\linewidth,keepaspectratio]{./assets/bf_qual/output_3_11.png}
  \includegraphics[width=0.45\linewidth,keepaspectratio]{./assets/bf_qual/output_3_12.png}
  \includegraphics[width=0.45\linewidth,keepaspectratio]{./assets/bf_qual/output_3_13.png}
  %\label{}
\end{figure}
\begin{figure}[!htbp]
  \centering
  \includegraphics[width=0.9\linewidth,keepaspectratio]{./assets/bf_qual/output_3_14.png}\\
  \includegraphics[width=0.45\linewidth,keepaspectratio]{./assets/bf_qual/output_3_15.png}
  \includegraphics[width=0.45\linewidth,keepaspectratio]{./assets/bf_qual/output_3_16.png}
  \includegraphics[width=0.45\linewidth,keepaspectratio]{./assets/bf_qual/output_3_17.png}
  \includegraphics[width=0.45\linewidth,keepaspectratio]{./assets/bf_qual/output_3_18.png}
  \includegraphics[width=0.45\linewidth,keepaspectratio]{./assets/bf_qual/output_3_19.png}
  \includegraphics[width=0.45\linewidth,keepaspectratio]{./assets/bf_qual/output_3_20.png}
  %\label{}
\end{figure}
\begin{figure}[!htbp]
  \centering
  \includegraphics[width=0.9\linewidth,keepaspectratio]{./assets/bf_qual/output_3_21.png}\\
  \includegraphics[width=0.45\linewidth,keepaspectratio]{./assets/bf_qual/output_3_22.png}
  \includegraphics[width=0.45\linewidth,keepaspectratio]{./assets/bf_qual/output_3_23.png}
  \includegraphics[width=0.45\linewidth,keepaspectratio]{./assets/bf_qual/output_3_24.png}
  \includegraphics[width=0.45\linewidth,keepaspectratio]{./assets/bf_qual/output_3_25.png}
  \includegraphics[width=0.45\linewidth,keepaspectratio]{./assets/bf_qual/output_3_26.png}
  \includegraphics[width=0.45\linewidth,keepaspectratio]{./assets/bf_qual/output_3_27.png}
  %\label{}
\end{figure}
\begin{figure}[!htbp]
  \centering
  \includegraphics[width=0.9\linewidth,keepaspectratio]{./assets/bf_qual/output_3_28.png}\\
  \includegraphics[width=0.45\linewidth,keepaspectratio]{./assets/bf_qual/output_3_29.png}
  \includegraphics[width=0.45\linewidth,keepaspectratio]{./assets/bf_qual/output_3_30.png}
  \includegraphics[width=0.45\linewidth,keepaspectratio]{./assets/bf_qual/output_3_31.png}
  \includegraphics[width=0.45\linewidth,keepaspectratio]{./assets/bf_qual/output_3_32.png}
  \includegraphics[width=0.45\linewidth,keepaspectratio]{./assets/bf_qual/output_3_33.png}
  \includegraphics[width=0.45\linewidth,keepaspectratio]{./assets/bf_qual/output_3_34.png}
  %\label{}
\end{figure}
\begin{figure}[!htbp]
  \centering
  \includegraphics[width=0.9\linewidth,keepaspectratio]{./assets/bf_qual/output_3_35.png}\\
  \includegraphics[width=0.45\linewidth,keepaspectratio]{./assets/bf_qual/output_3_36.png}
  \includegraphics[width=0.45\linewidth,keepaspectratio]{./assets/bf_qual/output_3_37.png}
  \includegraphics[width=0.45\linewidth,keepaspectratio]{./assets/bf_qual/output_3_38.png}
  \includegraphics[width=0.45\linewidth,keepaspectratio]{./assets/bf_qual/output_3_39.png}
  \includegraphics[width=0.45\linewidth,keepaspectratio]{./assets/bf_qual/output_3_40.png}
  \includegraphics[width=0.45\linewidth,keepaspectratio]{./assets/bf_qual/output_3_41.png}
  %\label{}
\end{figure}
\begin{figure}[!htbp]
  \centering
  \includegraphics[width=0.9\linewidth,keepaspectratio]{./assets/bf_qual/output_3_42.png}\\
  \includegraphics[width=0.45\linewidth,keepaspectratio]{./assets/bf_qual/output_3_43.png}
  \includegraphics[width=0.45\linewidth,keepaspectratio]{./assets/bf_qual/output_3_44.png}
  \includegraphics[width=0.45\linewidth,keepaspectratio]{./assets/bf_qual/output_3_45.png}
  \includegraphics[width=0.45\linewidth,keepaspectratio]{./assets/bf_qual/output_3_46.png}
  \includegraphics[width=0.45\linewidth,keepaspectratio]{./assets/bf_qual/output_3_47.png}
  \includegraphics[width=0.45\linewidth,keepaspectratio]{./assets/bf_qual/output_3_48.png}
  %\label{}
\end{figure}

\clearpage

\subsection{Breakfast Meta-test Set - Triplet Network Deatiled Alignment Analysis}

\begin{figure}[!htbp]
  \centering
  \includegraphics[width=0.9\linewidth,keepaspectratio]{./assets/bf_qual/output_4_0.png}\\
  \includegraphics[width=0.45\linewidth,keepaspectratio]{./assets/bf_qual/output_4_1.png}
  \includegraphics[width=0.45\linewidth,keepaspectratio]{./assets/bf_qual/output_4_2.png}
  \includegraphics[width=0.45\linewidth,keepaspectratio]{./assets/bf_qual/output_4_3.png}
  \includegraphics[width=0.45\linewidth,keepaspectratio]{./assets/bf_qual/output_4_4.png}
  \includegraphics[width=0.45\linewidth,keepaspectratio]{./assets/bf_qual/output_4_5.png}
  \includegraphics[width=0.45\linewidth,keepaspectratio]{./assets/bf_qual/output_4_6.png}
  %\label{}
\end{figure}

\begin{figure}[!htbp]
  \centering
  \includegraphics[width=0.9\linewidth,keepaspectratio]{./assets/bf_qual/output_4_7.png}\\
  \includegraphics[width=0.45\linewidth,keepaspectratio]{./assets/bf_qual/output_4_8.png}
  \includegraphics[width=0.45\linewidth,keepaspectratio]{./assets/bf_qual/output_4_9.png}
  \includegraphics[width=0.45\linewidth,keepaspectratio]{./assets/bf_qual/output_4_10.png}
  \includegraphics[width=0.45\linewidth,keepaspectratio]{./assets/bf_qual/output_4_11.png}
  \includegraphics[width=0.45\linewidth,keepaspectratio]{./assets/bf_qual/output_4_12.png}
  \includegraphics[width=0.45\linewidth,keepaspectratio]{./assets/bf_qual/output_4_13.png}
  %\label{}
\end{figure}
\begin{figure}[!htbp]
  \centering
  \includegraphics[width=0.9\linewidth,keepaspectratio]{./assets/bf_qual/output_4_14.png}\\
  \includegraphics[width=0.45\linewidth,keepaspectratio]{./assets/bf_qual/output_4_15.png}
  \includegraphics[width=0.45\linewidth,keepaspectratio]{./assets/bf_qual/output_4_16.png}
  \includegraphics[width=0.45\linewidth,keepaspectratio]{./assets/bf_qual/output_4_17.png}
  \includegraphics[width=0.45\linewidth,keepaspectratio]{./assets/bf_qual/output_4_18.png}
  \includegraphics[width=0.45\linewidth,keepaspectratio]{./assets/bf_qual/output_4_19.png}
  \includegraphics[width=0.45\linewidth,keepaspectratio]{./assets/bf_qual/output_4_20.png}
  %\label{}
\end{figure}
